# Supplementary material for: ZipperChain: Transmuting Trusted Third-Party Services Into Trustless Atomic Broadcast
Source: arXiv:2511.21969 source file (2025-11-26)
Supplement: Supplementary file 1 [file durability.tex]

\subsection{Durability}
\label{sec:appendix:durability}

\todo{copied from Colaboratory~\cite{22ZipperChainDurability} and made to compile - needs review}

We implement the ZipperChain Replication Service based on the correctness guarantees of Write Once, Read Many~(WORM) cloud storage systems.
WORM systems enable their clients to protect stored data against inadvertent modification, or deletion, to meet regulatory requirements on data retention~\cite{https://www.sec.gov/rules/interp/34-47806.htm}.
Specifically, the
AWS Simple Storage Service~(S3)~\cite{https://docs.aws.amazon.com/AmazonS3/latest/userguide/object-lock-overview.html},
Microsoft Azure Blob Storage~\cite{https://docs.microsoft.com/en-us/azure/storage/blobs/immutable-legal-hold-overview},
and Google Cloud Storage~\cite{https://cloud.google.com/storage/docs/bucket-lock}
guarantee object \emph{immutability} through legal/compliance holds on data objects that prevent anyone, including the bucket owner, from deleting or modifying objects.
Amazon~\cite{https://docs.aws.amazon.com/AmazonS3/latest/userguide/DataDurability.html},
Microsoft~\cite{https://docs.microsoft.com/en-us/azure/storage/common/storage-redundancy},
and Google~\cite{https://cloud.google.com/blog/products/storage-data-transfer/understanding-cloud-storage-11-9s-durability-target}
also design these services to provide 11 nines of \emph{durability} by replicating data across availability zones within a region.
Cloud storage providers allow, with some custom configuration, to make bucket settings publicly readable, which allows anyone to \emph{verify} that object holds are enabled.
Finally,
Amazon~\cite{https://aws.amazon.com/s3/sla/},
Microsoft~\cite{https://azure.microsoft.com/en-us/support/legal/sla/storage/v1\_5/},
and Google~\cite{https://cloud.google.com/storage/sla}
service level agreements~(SLAs) guarantee monthly 3-nines of **availability**, subject to financial penalties, which means less than 44 minutes of downtime.

\subsubsection{ZipperChain Durability On A Single Cloud Bucket}

Although the 11-nines durability guarantee is the industry standard, it is not sufficient by itself for storage of ZipperChain objects.
Let us see why.

ZipperChain stores $o = 4$ objects per block and we plan to push ZipperChain performance to the interval $i$ between blocks of $0.1$ seconds.
If we assume that we want a ZipperChain blockchain to operate for a 100 years that means that the blockchain will generate
$$
b = 100 \text{ years} \mult \frac{31536000 \text{ seconds}}{\text{year}} \mult \frac{\text{block}}{i \text{ seconds}} = 3.15\!\mult\!10^{10} \text{ blocks}
$$
blocks and $o \mult b$ objects.

For a ZipperChain to remain viable all the objects generated in each period must remain accessible.
11-nines of cloud durability allows us to define $a_c$ the annual failure rate~(AFR) of cloud objects as
$a_c = 1\!\mult\!10^{-11}$.
We transform it to a cloud object failure rate $f_c$ within a given block interval $i$ as
$$
f_c = F(a_c, i) =
a_c \frac{\text{failures}}{\text{year}} \mult
\frac{1 \text{ year}} {31536000 \text{ seconds}} \mult
\frac{i \text{ seconds}} {\text{block}}
= 3.17\!\mult\!10^{-20} \frac{\text{failures}}{\text{block}}
$$

Using the
Poisson distribution~\cite{https://en.wikipedia.org/wiki/Poisson\_distribution}
we
derive~\cite{https://github.com/Backblaze/erasure-coding-durability/blob/master/calculation.ipynb}
the probability $p_c$ of one or more failures in a period as $p_c = P(f_c) = 1 - e^{-f_c}$.
Considering that $f_c$ is very small, the difference between $p_c$ and $f_c$ is also small.
$$f_c - p_c = 5.03\!\mult\!10^{-40}$$

Finally, we calculate the cumulative durability $d^\text{*}_z$ of ZipperChain objects on a single cloud storage bucket as the probability of losing no objects created in the first period $(1-p_c)^o$, no object created in the first or second period $(1-p_c)^{2o}$, etc.
For all the periods $b$ we calculate the probability of not losing any objects as
$$
d^\text{*}_z = D^\text{*}\!(p_c, o, b) =
(1-p_c)^o \mult (1-P_C)^{2o} \mult \ldots \mult (1-P_C)^{bo} = \\
(1-p_c)^{o + 2o + \ldots + bo} =\\
(1-p_c)^{o \mult (1 + 2 + \ldots + b)} =\\
(1-p_c)^{o \mult \left((b+1) \mult \frac{b}{2}\right)} = \\
4.06\!\mult\!10^{-28}
$$
Clearly, this is woefully insufficient

\subsubsection{Cloud Storage Durability}

To understand how the ZipperChain Replication Service provides a more durable chain storage, we first must consider how cloud storage providers achieve durability.

An analysis by Backblaze~\cite{https://www.backblaze.com/blog/cloud-storage-durability/}
shows the utility of Reed-Solomon erasure codes in addressing disk failures.
They define a prototypical storage configuration with an annual disk failure rate $a_s = 0.405\%$ and a disk recovery period $r_s = 6.5\text{ days}$ based on an estimate of disk recovery rate of $12 \frac{\text{terabytes}}{\text{day}}$.
To mitigate the impact of disk failures, cloud storage providers encode an object into $n_c$ shards, including $k_c$ parity shards, and store them on independent disks.
As long as at least $n_c - k_c$ shards remain the object may be decoded.
Backblaze gives a typical configuration of $n_c=20$ and $k_c=3$.
Using the previously defined functions we calculate the probability $p_s$ of a shard being lost due to a failure of a disk as
$$
p_s = P \left( F \left(a_s, r_s \mult \frac{86400 \text{ seconds}}{\text{day}}\right)\right) = 7.21\!\mult\!10^{-5}
$$

Given the probability of a shard failing, we can use the
binomial distribution~\cite{https://en.wikipedia.org/wiki/Binomial_distribution}
probability mass function~(PMF) to calculate the probability of $k_c$ out of $n_c$ shards failing.
$$
{n_c \choose k_c} {p_s}^{k_c} \,\, (1 - p_s)^{n_c - k_c}
$$

However, an object is lost if $k_c + 1$ or more shards fail.
We calculate the joint probability of these failures using the binomial cumulative distribution function~(CDF).
$$
\text{CDF}_S = \sum_{j=k_c + 1}^{n_c} {n_c \choose j} {p_s}^j \,\, (1 - p_s)^{n_c - j}
= 1.31\!\times\!10^{-13}
$$

Finally, the durability of an object over the recovery period $r_s$ is $1 - \text{CDF}_s$ and its durability over a year is
$$
d_c = (1 - \text{CDF}_s)^{365 \frac{\text{days}}{\text{year}} / r_s \text{days} } = 0.999999999993
$$
or 11-nines.

To simplify further discussion, we define an object durability function $D(a, r, n, k)$, which aggregates the steps of the object durability calculation.

\subsubsection{ZipperChain Durability With The Replication Service}

To increase the probability that a ZipperChain chain remains viable, we apply erasure coding to ZipperChain objects to distribute their storage.
Using random linear network coding~(RLNC)~\cite{Ho2006Random}
the ZipperChain Replication Service encodes each object into $n_z = 6$ shards including $k_z = 3$ redundant shards.
We partition these shards across $n_z$ buckets located in different cloud storage providers and regions, which allows us to assume independence of bucket failures.

One key difference between the ZipperChain Replication Service and a cloud storage replication service is the time of replica recovery.
$r_s$ of $6.5 \text{ days}$ makes sense in relation to the size of a disk.
We need to define, $r_z$ based on the amount of data ZipperChain stores in each cloud bucket and the transfer rates between buckets.
The ZipperChain implementation uses $1,\!328 \text{ bytes}$
for the $o$ objects required for each block.
% <!--
% - header (block + timestamp attestation) - 1202B
% - tree - 54B
% - sequence - 32*2 + 8 = 72
% - totoal = 1202+54+72 = 1328
% -->

With the conservative assumptions that all $ob$ objects generated over the 100 years of operation exist in year one and with a conservative one-connection estimate of inter-region transfer speed~\cite{https://medium.com/slalom-technology/examining-cross-region-communication-speeds-in-aws-9a0bee31984f}
is $160 \text{ Mbps}$
we calculate the time $r_z$ to recover the state of a bucket user by ZipperChain as
$$
r_z = 1328 \frac{\text{bytes}}{\text{block}}
\mult \frac{\text{block}}{o \text{ objects}}
\mult \frac{b \text{ objects}}{(n_z - k_z) \text{ buckets}}
\mult 8 \frac{\text{bits}}{\text{byte}}
\mult \frac{1 \text{Mb}}{ 1\!\mult\!10^6 \text{ bits}}
\mult \frac{1 \text{ second}}{ 160 \text{ Mb}}
= 1.74\!\mult\!10^5 \frac{\text{seconds}}{\text{bucket}}
$$
or about $48 \text{ hours}$.

Given these constants, we calculate the durability $d_z$ of a ZipperChain object as
$$
d_z = D(1-d_c, r_z, n_z, k_z) \implies 35 \text{ nines}
$$

The 35-nines of object reliability achieved by the ZipperChain Replication service is a marked improvement over the 11-nines of cloud storage reliability.
But how do 35-nines of object durability translate to the probability that a ZipperChain chain remains viable over a 100 year period?

To answer that question we use the cumulative durability function $D^\text{*}$.
Plugging in the probability of object failure $1 - d_z$, the number of ZipperChain objects $o$ created for each block, and the number of $b$ we get
$$
d^\text{*}_z = 0.9999999999999903
$$
or 14-nines of cumulative durability.

Thus with the ZipperChain Replication Service our users may trust that the ZipperChain chain retains \emph{durability}, because with high probability its objects will not be lost through disk, or storage provider failure.
Users may also \emph{verify} through exposed cloud service configurations the level of replication and that each bucket has legal/compliance holds enabled to guarantee object \emph{immutability}.
