# Supplementary material for: ZipperChain: Transmuting Trusted Third-Party Services Into Trustless Atomic Broadcast
Source: arXiv:2511.21969 source file (2025-11-26)
Supplement: Supplementary file 2 [file immutability.tex]

\subsection{Immutability}
\label{sec:appendix:immutability}

\begin{definition}[Identifies]
Given the identification operator `$\,\ids\,$' and two data structures $x$ and $y$, $x \ids y \iff$ $x$ contains a reference to $y$.
\end{definition}
\noindent
Without loss of generality, if $y$ is a member of $x$ then $x$ \emph{identifies} the value of $y$, or in other words $x.y \implies x \ids y$.

\begin{definition}[Hashes]
Given the hashing operator `$\,\,\hashes\,$' and two data structures $x$ and $y$, $x \hashes y \iff x \ids \hash(y)$.
\end{definition}

\begin{definition}[Signs]
Given the signing operator `$\,\,\signs\,$' and two data structures $x$ and $y$, $x \!\!\underset{K}{\signs}\!\! y \iff x \ids \encrypt{K^-}{\hash(y)}$.
For convenience, the underset key may be omitted. 
\end{definition}

\begin{theorem}
    Given,
        a set $\zpr$ of on main chain triads,
        \timesvclong\ public key $\key^+_\timesvc$,
        \seqsvclong\ public key $\key^+_\seqsvc$,
    the hash and order of a transaction $\tx \in \zpr$ remains signed by the \timesvclong\ private key $\key^-_\timesvc$ and by the \seqsvclong\ private key $\key^-_\seqsvc$.
\end{theorem}

\begin{proof}
We will show by induction ...

Base case:

Let $\tri_0 = \zpr[0]$.
Since $\tri_0$ is part of \omc\ output, we know that $\tri_0$ is a true triad.
In a true triad $\time \signs \block$, $\seq \uids \block$, and $\seq \usigns \time$.

Let $\tri$ be true triad $\langle \block, \time, \seq \rangle$.
By the construction of $\time$ we know that $\time \signs \block$.
Similarly, we know by the construction of $\seq$ that $\seq \uids \block$ and $\seq \usigns \time$.
$a \uhashes b$

From the construction process of blocks, we know that there is a one to one relationship between
\end{proof}
