# Supplementary material for: ZipperChain: Transmuting Trusted Third-Party Services Into Trustless Atomic Broadcast
Source: arXiv:2511.21969 source file (2025-11-26)
Supplement: Supplementary file 3 [file agreement.tex]

\subsection{Agreement}
\label{sec:appendix:agreement}
