# Supplementary material for: ZipperChain: Transmuting Trusted Third-Party Services Into Trustless Atomic Broadcast
Source: arXiv:2511.21969 source file (2025-11-26)
Supplement: Supplementary file 4 [file availability.tex]

\subsection{\sol\ Availability}
\label{sec:appendix:availability}

As mentioned earlier, a key aspect of a stable storage is its availability, or the guarantee that users can retrieve stored objects within some time bound.
The ZipperChain Replication Service encodes each object into $n_z=6$  shards including $k_z=3$ redundant shards, which means that to retrieve (and decode) an object a user must collect any $n_z - k_z = 3$ shards.
Also as mentioned earlier the availability $a_c$ guaranteed by cloud storage providers is $a_c = 99.9\%/\text{month}$.
Again, since ZipperChain objects reside on buckets in different regions, we assume independence of unavailability.
With these numbers we calculate the availability $a_z$ of a ZipperChain object as
$$
a_z = 1 - \sum_{j\, =\, n_z - k_z + 1}^{n_z} {n_z \choose j} (1-a_c)^j \,\, (a_c)^{n_z - j}
= \frac{99.999999999\%}{\text{month}},
$$
or less than $0.0003 \text{ milliseconds}$.

That number, while impressive, can be somewhat misleading.
While placing data on different buckets allows us to assume independent durability failures, the availability of data in multiple buckets may, to a degree, be plagued by same problems such as a wide-scale power outage.
So, in the worst case the unavailability of the different buckets could line up bringing $a_z$ to $99.9\% / \text{month}$.
