# Supplementary material for: ZipperChain: Transmuting Trusted Third-Party Services Into Trustless Atomic Broadcast
Source: arXiv:2511.21969 source file (2025-11-26)
Supplement: Supplementary file 5 [file VPBS_and_other_old_stuff.tex]

% The goal of \sol\ is to provide correctness guarantees on par with other blockchain implementations, namely \emph{immutability}, \emph{agreement}, and \emph{availability}.
% While there exists a considerable variety in blockchain protocols, for many we can define the state of a blockchain as a totally ordered ledger of transactions.
% Any node may execute these transactions in that order to obtain a key-value store representing the values of token accounts and smart contract variables.
% This perspective on blockchains allows us to specify the correctness guarantees as follows:
% \begin{itemize}
%     \item \textbf{Blockchain-Immutability} -- If a valid quorum node has a transaction at some position in its ledger, it will continue to have that transaction at that position in its ledger.
%     \item \textbf{Blockchain-Agreement} -- If a valid quorum node has a transaction at some position in its ledger, all valid quorum nodes will have that transaction at that position and only that position in their ledgers.
%     \item \textbf{Blockchain-Availability} -- The quorum of valid nodes remains valid.
%     % , which implies that all nodes are never replaced simultaneously, which allows the state to persist...
% \end{itemize}
% Note that Blockchain-Availability implies that all nodes of a quorum are never replaced simultaneously, which allows the state of the blockchain to persist.
% Additionally, Blockchain-Availability may also be considered to provide liveness, where, barring network partitions, a user may always write to and read transactions from the blockchain.
% Finally, the quorum in many blockchains is a qualified majority.

% \begin{table}[h]
%     \centering
%     \begin{tabular}{l|l}
%     \hline
%     Symbol & Meaning \\
%     \hline
%      $\val$ & Consensus value \\

%     $\slot$ & Execution timeslot \\
%     $\slots$ & A set of execution timeslots (execution timeline) \\

%     $\user$ & \userlong \\
%     $\users$ & A set of \userlong s \\

%     \hline
%     \end{tabular}
%     \vspace{5pt}
%     \caption{Additional notation complementing \reftbl{tbl:notation}.}
%     \label{tbl:additional_notation}
% \end{table}

% A blockchain can also be viewed as an implementation of a multi-round Validity Predicate-based Byzantine Consensus~(VPBC)~\cite{Crain18DBFT}.
% Nodes running a VPBC protocol decide on a value $\val$\footnotemark\ that satisfies a predicate $\valid()$.
% \footnotetext{To aid the discussion of \sol\ correctness guarantees we introduce additional notation summarized in \reftbl{tbl:additional_notation}}
% In the context of blockchains $\valid(\val)$ enforces structural properties such as cryptographic links between blocks, or that transactions are not malformed.
% The correctness guarantees in each round of VPBC are:
% \begin{itemize}
%     \item \textbf{VPBC-Validity} -- A non-faulty process decides on $\val$ only if a non-faulty process proposed $\val$ and if $\valid(\val)$ is true.
%     \item \textbf{VPBC-Agreement} -- No two non-faulty processes decide on different values.
%     \item \textbf{VPBC-Integrity} -- Each process decides on a value at most once.
%     \item \textbf{VPBC-Termination} -- Every non-faulty process eventually decides on a value.
% \end{itemize}
% To ensure that a VPBC protocol produces a total order of transactions, we define the predicate $\valid(\val)$ to return true if $\val$ is a non-malformed transaction and no node decides on $\val$ in any previous round.
% A VPBC protocol may also assume that node storage is stable, that each round is decided by a quorum of nodes, there is a non-zero overlap between quorums in each round, and that more than two-thirds of nodes in each round are honest.
% Under these assumptions a correct VPBC protocol satisfies blockchain correctness guarantees as
% Blockchain-Immutability is satisfied by VPBC-Integrity and the stable storage assumption,
% Blockchain-Agreement is satisfied by VPBC-Validity and VPBC-Agreement,
% finally, the persistent state guaranteed by Blockchain-Availability is satisfied by the stable storage, quorum overlap, and two-thirds honest assumptions.

% It is worthwhile to note that no consensus protocol providing validity, agreement, integrity, and termination is possible under message loss, or node failure~\cite{Akkoyunlu75TwoGenerals, Fischer85Impossibility}.
% To get around this impossibility result consensus protocols can
% deterministically reach probabilistic consensus, as in Bitcoin~\cite{Nakamoto08Bitcoin},
% or reach consensus probabilistically by guaranteeing termination if certain conditions in terms of message delivery to non-faulty processes have been met~\cite{Buchman19Tendermint, Crain18DBFT}.

% To demonstrate the correctness of \sol, we
% define its correctness guarantees in terms of VPBC validity, agreement, integrity, and termination,
% prove that the \sol\ protocol provides these properties,
% and finally map these properties to blockchain immutability, agreement, and availability.

% \subsection{\sol\ correctness guarantees}

% To define \sol's correctness guarantees we assume the execution of the \sol\ protocol can be discretized into a set $\slots$ of infitesimally small time slots.
% We also assume a set of \userlong s $\users$ and a \sol\ deployment $\zeta$.
% We define \sol's correctness guarantees as follows:
% \vspace{7pt}
% \begin{itemize}
%     \item
%     \textbf{\sol-Validity} --
%     A transaction $\tx$ can be finalized on a \sol\ blockchain only if some \userlong\ has submitted it.
%     In other words, a \sol\ user can obtain a certificate for a transaction, only if there is a user that has submitted that transaction at an earlier time.
%     Formally,
%     \[
%     \forall \user, \user' \in \users, \slot, \slot', \slot'' \in \slots,
%     \user'\!.\verify_{\slot''}(\tx) \!\rightarrow\! \cert
%     \implies
%     \user.\writef_\slot(\tx) \land \zeta.\writef_{\slot'}(\tx) \land \slot < \slot' < \slot''
%     \]

%     \todo{revise below}

%     \item
%     \textbf{Safety} -- Once $\tx$ is finalized, it will remain finalized,\footnotemark\ or
%     \[
%     (\text{\verify}(\tx) \!\rightarrow\! \cert) \implies \mathcal{G}\, (\text{\verify}(\tx) \!\rightarrow\! \cert)
%     \]
%     \footnotetext{We define the safety property using Linear Temporal Logic.}


%     \item
%     \textbf{Agreement} -- If one correct \userlong\ obtains a certificate then all correct \userlong's obtain the same certificate, or
%     \[
%     \forall \tx, \tx', \cert, \cert', (\text{\verify}(\tx) \!\rightarrow\! \cert) \land (\text{\verify}(\tx') \!\rightarrow\! \cert') \implies \tx = \tx' \land \cert = \cert'
%     \]


%     \item
%     \textbf{Liveness} -- If a process keeps resubmitting $\tx$, it will eventually become finalized, or
%     \[
%     (\text{\verify}(\tx) \!\rightarrow\! \cert) \,\mathcal{M}\, \text{\writef}(\tx)
%     \]
% \end{itemize}

% The safety property is related to the immutability property.
% While safety defines the behavior of the \verify\ function, immutability defines the behavior of data stored on the blockchain.
% The safety property is also related to availability.
% Safety implies that a user may always execute the \verify\ function, which depends on the availability of the \repsvclong.
% Note that \sol\ does not guarantee that a \userlong\ may always execute the \writef\ function to record new transactions.
% Finally, agreement in blockchains is generally understood to imply a total order over transactions.
% Since \sol\ certificates include the position of the transaction in a block on the main chain, agreement over certificates also implies agreement over order.

% \todo{revise below}


% \subsection{System model}

% To prove that \sol, as a consensus protocol, provides the aforementioned correctness guarantees, we first need to define our assumptions about the system model.
% Specifically, we assume that:

% \begin{enumerate}
% \item The instantiations of the \timesvclong, the \seqsvclong, and the \repsvclong\ do not fail permanently.
% This assumption is reasonable because the \timesvclong\ and the \repsvclong\ are themselves distributed services with uptime guarantees.
% The \seqsvclong, on the other hand, is executed in a \sol\ deployment on a single machine.
% We have a solution for a reliable replacement of a \seqsvclong\ instantiation that we will present and prove in a follow-up paper.

% \item We assume that an object replicated by the \repsvclong\ remains accessible and, specifically, that at least one correct copy of the object my be downloaded by a \userlong.
% This assumption is reasonable, because the \repsvclong\ is distributed and the objects are stored on a large number of independent nodes.
% It is therefore as unlikely that objects in the \repsvclong\ would become unavailable as it is for data to become unavailable in a network of public blockchain miners.



% \end{enumerate}



% % We proceed the correctness properties of \sol\ with a proof by invariants.
% % Invariants are predicates about a system that hold true at all points of system execution.
% % We first define a set of invariants about \sol, then prove them, and finally use the invariants to prove \sol\ correctness guarantees.

% \subsection{Safety}

% \todo{Bear pointed out a limitation of the system where we could have a collision on two timestamp attestations and we wouldn't know which one was correct. So someone could hold back an earlier one and then produce it later to move up the timestamp of a block.}

% \todo{This is an outline of the proof - needs to be made tighter after we review the correctness of the \verify\ mechanism.}

% We defined safety as
% \[
% (\text{\verify}(\tx) \!\rightarrow\! \cert) \implies \mathcal{G}\, (\text{\verify}(\tx) \!\rightarrow\! \cert).
% \]
% We assume that objects written to the \repsvclong\ cannot be erased, and so we can redefine safety as

% \begin{theorem}
% \label{thm:safety}
% \begin{align*}
% \exists\, \blocks, \times, \encls ~|~ \cert = \text{\verify}(\tx)
% \implies
% \forall\, \blocks' \supseteq \blocks, \times' \supseteq \times, \encl' \supseteq \encls,  \cert = \text{\verify}(\tx)
% \end{align*}
% \end{theorem}

% \noindent
% where once $\text{\verify}(\tx)$ returns $\cert$ based on some sets of blocks~$\blocks$, timestamp attestations~$\times$, and enclave attestations~$\encls$ it will continue to do so regardless of what objects are added to $\blocks, \times, \encls$ to form $\blocks'\!, \times'\!, \encls'$.

% \begin{proof}
% We prove \refthm{thm:safety} by induction.

% \noindent
% Base case: $\blocks' = \blocks, \times' = \times, \encls' = \encls$

% There either exist $\blocks, \times, \encls$ such that \verify\ returns a certificate, or not.
% So we can prove the base case by parts:
% \begin{itemize}
%     \item If the antecedent $\exists\, \blocks, \times, \encls ~|~ \cert = \text{\verify}(\tx)$ is true then
%     \begin{align*}
%     \exists\, \blocks, \times, \encls ~|~ \cert = \text{\verify}(\tx)
%     \implies
%     \vspace{20pt}\forall\, \blocks' \supseteq \blocks, \times' \supseteq \times, \encls' \supseteq \encls, \cert = \text{\verify}(\tx)\\
%     %
%     \top \implies \forall\, \blocks' \supseteq \blocks, \times' \supseteq \times, \encls' \supseteq \encls, \cert = \text{\verify}(\tx)
%     & &\text{by assumption}\\
%     %
%     \top \implies \forall\, \blocks, \times, \encls,  \cert = \text{\verify}(\tx)
%     & &\text{by substitution}\\
%     %
%     \top \implies \top && \text{since $\blocks, \times, \encls$ fixed}\\
%     %
%     \top
%     \end{align*}

%     \item If the antecedent $\exists\, \blocks, \times, \encls ~|~ \cert = \text{\verify}(\tx)$ is false then
%     \begin{align*}
%     \exists\, \blocks, \times, \encls ~|~ \cert = \text{\verify}(\tx)
%     \implies
%     \vspace{20pt}\forall\, \blocks' \supseteq \blocks, \times' \supseteq \times, \encls' \supseteq \encls, \cert = \text{\verify}(\tx)\\
%     %
%     \bot \implies \forall\, \blocks' \supseteq \blocks, \times' \supseteq \times, \encls' \supseteq \encls, \cert = \text{\verify}(\tx)
%     & &\text{by assumption}\\
%     %
%     \top
%     \end{align*}
% \end{itemize}

% \noindent
% Inductive hypothesis: Suppose \refthm{thm:safety} holds for some $\blocks, \times, \encls$.

% \noindent
% Inductive step: Extend $\blocks, \times, \encls$ with another object -- block, timestamp attestation, or enclave attestation.
% Formally, assume any $\blocks' \supseteq \blocks$, $\times' \supseteq \times$, and $\encls' \supseteq \encls$ and in each step let either
% $\blocks = \blocks \cup \{\block'\} \ni \block' \in \blocks'$,
% $\times = \times \cup \{\time'\} \ni \time' \in \times'$,
% or $\encls = \encls \cup \{\encl'\} \ni \encl' \in \encls'$.
% Several cases are possible:
% \begin{itemize}
%     \item The new object is a duplicate, in which case the state of $\blocks, \times, \encls$ does not change and \refthm{thm:safety} holds after the inductive step by the inductive hypothesis.

%     \item The new object does not change the set $\succs$ on line~\ref{alg:omc:succs} in \refalg{alg:omc} at any point in its execution.
%     That means that the set $\encls^*$ on line~\ref{alg:omc:auths} remains unchanged as well.
%     Consequently the calls to \path\ on line~\ref{alg:omc:path} find no fewer paths.
%     As a result the execution flow and output of \omc\ does not change, the rest of \verify\ executes without change, and \refthm{thm:safety} holds after the inductive step.

%     \item The new object, possibly in combination with objects added in previously taken inductive steps, changes the set $\succs$ on line~\ref{alg:omc:succs} in \refalg{alg:omc} at some point in its execution.
%     For the change in $\succs$ to affect the main chain, line~\ref{alg:omc:auth} would need to produce $\underline{\encl}' < \underline{\encl}$.
%     However, since $\underline{\encl}$ is already the smallest element in $\succs$ that would be a contradiction, and so \refthm{thm:safety} holds after the inductive step.
% \end{itemize}

% So, \refthm{thm:safety} holds for the inductive step and by the principle of mathematical induction \refthm{thm:safety} holds.

% \end{proof}

% \subsection{Liveness}
% \label{sec:appendix:liveness}


% % \subsection{Immutability}

% % We want to show that once a transaction $\tx$ is written onto a \sol\ blockchain, it will remain on that blockchain.
% % Specifically to the implementation of \sol, once \verify$(\tx)$ returns a certificate $\cert$, it will always return that certificate over the correct blockchain and none over any other blockchain.

% % Assumptions:
% % \begin{itemize}
% %     \item The \sol\ blockchain is comprises only main chain blocks.
% %     \item The storage used by the \repsvclong\ is stable.
% %     In other words, items replicated by the \repsvclong\ remain retrievable from storage.
% %     \item Block zero for the \sol\ blockchain is well-known.
% % \end{itemize}

% % When the \verify\ function returns \true, it means that all the checks in the process described in \refsec{sec:implementation:verify} have passed.
% % That means that storage contains sets $\blocks, \merkles, \encls$ for which \verify$(\tx)$ returns \true.
% % Since storage is stable the elements of these sets cannot be deleted from storage.
% % An attacker may, however, add additional elements to these sets, which could contain modifications.

% % verify will return true for the original combinations
% % verify will return false for any other combination

% % prove by parts:
% % - attacker adds a $\merkle'$
% % - attacker adds a $\block'$
% % - attacker adds a $\time'$
% % - attacker adds a $\encl'$



% % conclude that it will fail because one of these elements has to be added first



% % \todo{\href{https://blocky.atlassian.net/browse/BKY-2345}{BKY-2345}}

% % % Timestamp is unfakable and immutable $\leftarrow$ by CA

% % % Data has is immutable $\leftarrow$ by CA

% % % Blocks cannot be inserted post fact $\leftarrow$ \ttt{prev\_CVB\_hash} prevents us from generating blocks out of order

% % % BLOCKY is the only one that can create CVL blocks $\leftarrow$ only BLOCKY has $K_{C}^-$ with $K_{C}^+$ signed by $K_{B}^-$

% % \subsection{Agreement}



% % \todo{\href{https://blocky.atlassian.net/browse/BKY-2346}{BKY-2346}}

% % \subsection{Availability}

% % \todo{we assume that this service cannot fail}

% % \todo{\href{https://blocky.atlassian.net/browse/BKY-2348}{BKY-2348}}

% % Storage of CVBs is reliable $\leftarrow$ replication?
